# Supplementary material for: Wasserstein Distributionally Robust Regret-Optimal Control in the Infinite-Horizon
Source: arXiv:2312.17376 source file (2023-12-28)
Supplement: Supplementary file 1 [file appendix_0_organization.tex]

\todo{organization of the appendix}
