# Supplementary material for: Wasserstein Distributionally Robust Regret-Optimal Control in the Infinite-Horizon
Source: arXiv:2312.17376 source file (2023-12-28)
Supplement: Supplementary file 2 [file appendix_1_definitions.tex]

\todo{definitions of the operators}

\begin{align}
    \Tfin_{\Kfin,T} \defeq \begin{bmatrix} \Ffin_{T} \Kfin_{T} + \Gfin_{T} \\ \Kfin_{T} \end{bmatrix}
\end{align}

\begin{equation}
    \Kfin_{\circ,T} \defeq - (\Ifin_T + \Ffin_{T}^\ast \Ffin_{T})^{\-1}\Ffin_{T}^\ast \Gfin_{T}
\end{equation}
