# Supplementary material for: Wasserstein Distributionally Robust Regret-Optimal Control in the Infinite-Horizon
Source: arXiv:2312.17376 source file (2023-12-28)
Supplement: Supplementary file 3 [file appendix_3_technical.tex]

\todo{asymptotically equaivalent matrices} \\
\todo{Szego theorems limit theorems}\\
\todo{Danskin's theorem}\\
\todo{Spectral theorem} \\
\todo{$\Gamma-$convergence}\\
\todo{Fatou's lemma with varying measure}
